# Supplementary material for: Standard Plane Detection in 3D Fetal Ultrasound Using an Iterative Transformation Network
Source: arXiv:1806.07486 ancillary file (2018-10-07)
Supplement: Supplementary file 1 [file Appendix.pdf]

## Appendix A Derivation of $\boldsymbol{c}^{GT}$ and $\boldsymbol{k}^{GT}$

$c^{GT}$ is computed by selecting the component of $\boldsymbol{t}^{GT}$ with the maximum absolute value and taking into account its sign,

$$c^{GT} = \begin{cases} c_i^+, & \text{if} \quad t_i^{GT} > 0 \\ c_i^-, & \text{otherwise.} \end{cases} \tag{2}$$

where $i = \text{argmax}(\text{abs}(\boldsymbol{t}^{GT}))$. For a vector $\boldsymbol{a}$, $\text{argmax}(\boldsymbol{a})$ returns the index of the vector component with maximum value.

$k^{GT}$ is computed by selecting the coordinate axis about which there is the largest rotation away from the GT plane. However, this cannot be determined directly from the quaternion $\boldsymbol{q}^{GT}$ since it cannot be broken down into individual rotations about each coordinate axis. We overcome this problem by converting quaternion to Euler angles which give a more intuitive sense of the amount of rotation about each axis. However, Euler angles are affected by the order of rotation and there are a total of 6 different conventions to represent Euler angles based on the order of rotation about x, y, z-axis. We denote these conventions as 'xyz', 'xzy', 'yxz', 'yzx', 'zxy', 'zyx' where 'xyz' means a rotation about x-axis followed by y-axis and finally z-axis. This again causes problem in determining the axis with largest rotation because different conventions may give rise to different axis with the largest rotation. To solve this problem, we convert $\boldsymbol{q}^{GT}$ to Euler angles using all 6 conventions which gives rise to 6 sets of 3 Euler angles. For each convention, we take only the first Euler angle (ie. angle of the first rotation) and collect them into a vector $\boldsymbol{\theta}^{GT} = (\theta_{xyz,1}, \theta_{xzy,1}, \theta_{yxz,1}, \theta_{yzx,1}, \theta_{zxy,1}, \theta_{zyx,1})$. For instance, $\theta_{xyz,1}$ denotes the first Euler angle when converting using 'xyz' convention and in this case, it gives the amount of rotation about the x-axis. Hence, for any rotation represented by $\boldsymbol{q}^{GT}$, $\boldsymbol{\theta}^{GT}$ breaks it down and gives a list of the possible angles of the first rotation about the three standard coordinate axes. This overcomes the problem of different rotation order since we are restricting our comparison to the first rotation angle. $k^{GT}$ can then be computed similar to $c^{GT}$ by selecting the component of $\boldsymbol{\theta}^{GT}$ with the maximum absolute value and taking into account its sign,

$$k^{GT} = \begin{cases} k_j^+, & \text{if} \quad \theta_i^{GT} > 0 \\ k_j^-, & \text{otherwise.} \end{cases} \tag{3}$$

where $i = \text{argmax}(\text{abs}(\boldsymbol{\theta}^{GT}))$ and $j = \lceil i/2 \rceil$. During inference, $\boldsymbol{Q}$ will then give an intuitive sense of the most likely axis about which the rotation should occur.

## Appendix B Network Architectures

Fig. 3 shows all the network architectures used for different CNN outputs. All networks comprise 5 convolution layers (C), each followed by a max-pooling layer (P). After the 5th pooling layer, the network branches into fully-connected

(FC) layers. The number of branches depends on the transformation representation. Fig. 3a shows the network for predicting anchor points $\boldsymbol{A}$. Fig. 3b shows the network for predicting translation $\boldsymbol{t}$ and rotation $\boldsymbol{r}$ represented by either quaternion ($n_r$=4), Euler angles ($n_r$=3) or rotation matrix ($n_r$=9). Fig. 3c shows the network for predicting translation $\boldsymbol{t}$ and quaternion $\boldsymbol{q}$ with classification probabilities $\boldsymbol{P}$ and $\boldsymbol{Q}$. Output size of each layer is represented as width × height × (# feature maps). All convolution layers use 3x3 kernel with stride=1 and all pooling layers use 2x2 kernel with stride=2. ReLU activation function is applied after all convolution and FC layers except for the last FC layer of each task. Drop-out is also added after each FC layer.

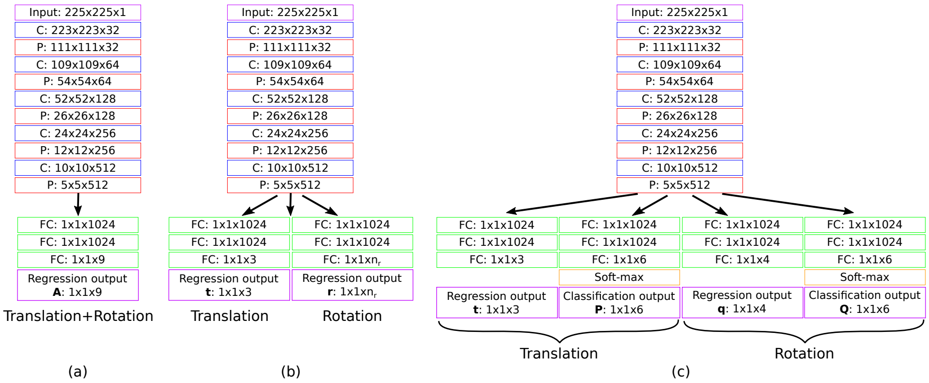


Fig. 3: Network architectures for (a) anchor points, (b) translation + quaternion/Euler angles/rotation matrix and (c) translation + quaternion with classification probabilities. Output size of each layer is represented as width × height × (# feature maps).
